# Supplementary material for: Scaling Laws for Hyperparameter Optimization
Source: arXiv:2302.00441 source file (2023-10-25)
Supplement: Supplementary file 1 [file appendix_algorithm.tex]

\section{Method Algorithm}
\label{app:method_algorithm}

\begin{algorithm}[ht!]

\SetAlgoLined
\SetKwInOut{Input}{Input}
\SetKwInOut{Output}{Output}
\Input{Search space $\Lambda$, initial design $H^{(0)}$, budget increment $b^{\text{step}}$}
\Output{Best hyperparameter configuration $\lambda^*$}
\smallskip
Evaluate initial configurations and budgets $H := H^{(0)}$ \;  \smallskip
 \While{still budget}{
 \smallskip
 Fit a DPL ensemble $\hat f^{(1)}(\lambda,b), \dots, \hat f^{(K)}(\lambda,b)$ from history $H$ using Equation~\ref{eq:powerlawobjective}\;
 \smallskip
 \smallskip
 Define the posterior mean and variance $\mu_{\hat f}(\lambda,b), \sigma^2_{\hat f}(\lambda,b)$ using Equation~\ref{eq:meanvar}\;
 \smallskip
 \smallskip
  Recommend the next configuration $\lambda^{\text{next}}$ using Equation~\ref{eq:acquisition}\;
 \smallskip 
 \smallskip
 Compute the next budget $b^{\text{next}}$ using Equation~\ref{eq:steps}\;
 \smallskip
 \smallskip
 \smallskip
 Train $\lambda^{\text{next}}$ until $b^{\text{next}}$ and measure the validation loss
 $f\left(\lambda^{\text{next}}, b^{\text{next}} \right)$\;
 \smallskip
 \smallskip
 Append to history $H \leftarrow H \cup \left\{\left(\lambda^{\text{next}}, b^{\text{next}}, f\left(\lambda^{\text{next}}, b^{\text{next}} \right)\right)\right\}$\;
 }
 \smallskip
\textbf{return} Best configuration $\lambda^*$ with the smallest validation loss  $\min\limits_{\left(\lambda^*, b, f\left(\lambda^*, b\right) \right) \in H } \; f\left(\lambda^*, b\right)$ \;
 \caption{Multi-Fidelity HPO with Deep Power Laws}
 \label{alg:grayboxhpo}
\end{algorithm}
